# Supplementary material for: Even denominator fractional quantum Hall states at an isospin transition in monolayer graphene
Source: arXiv:1712.01968 source file (2017-12-12)

# Measurement schematic for $C_p$

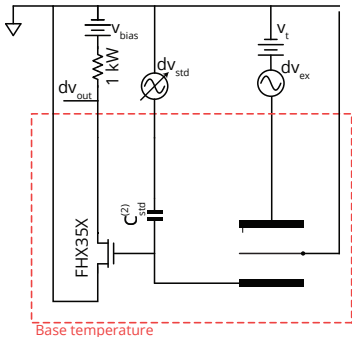

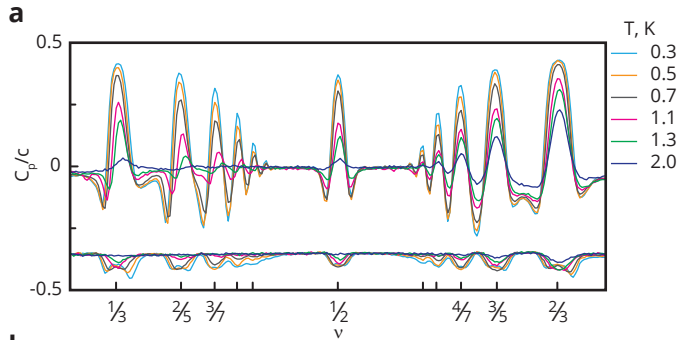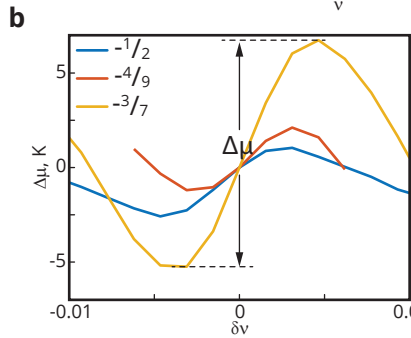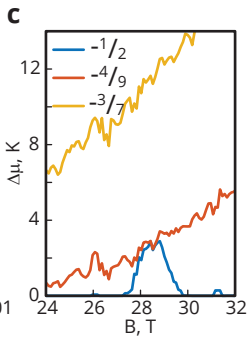

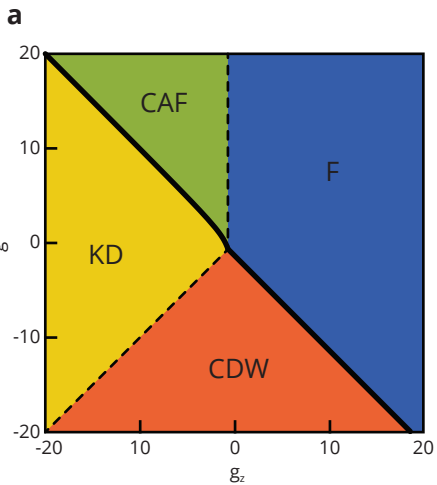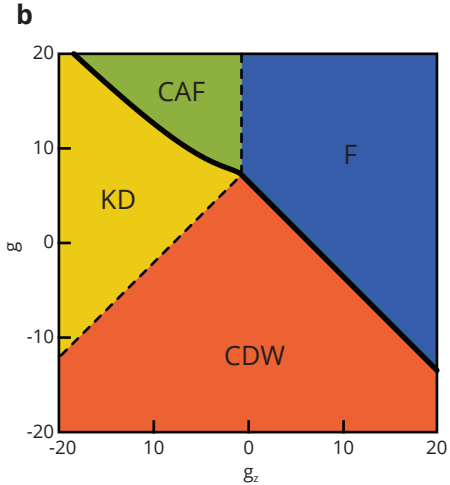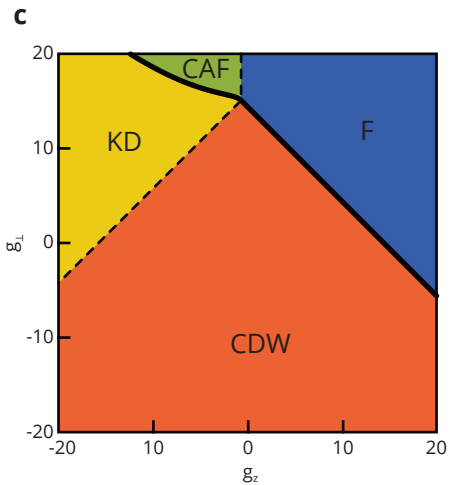

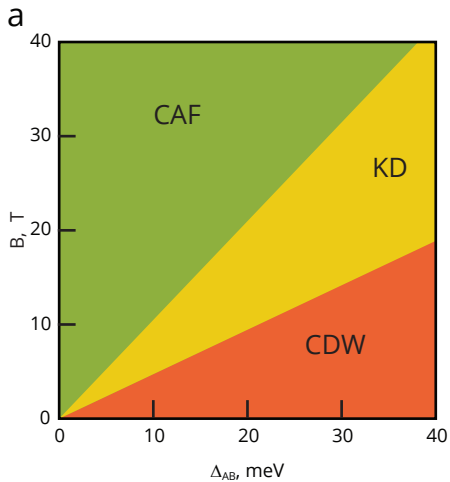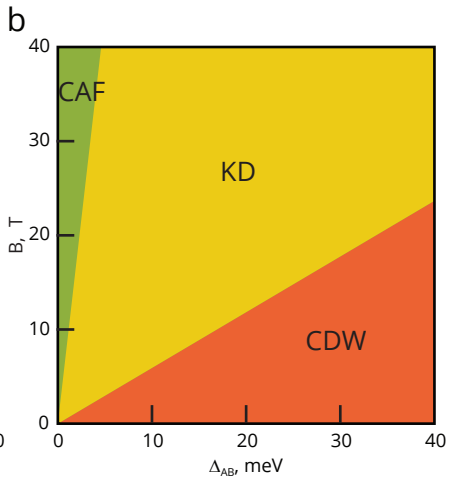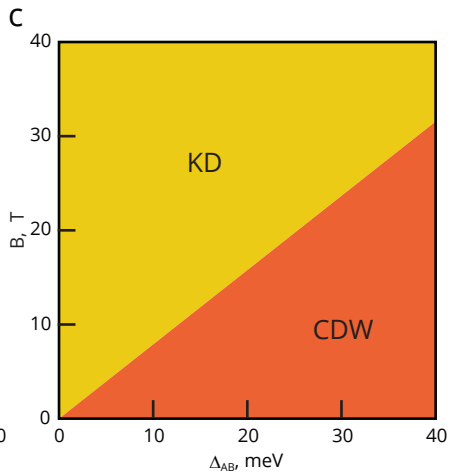

Sample D

T=20 mK

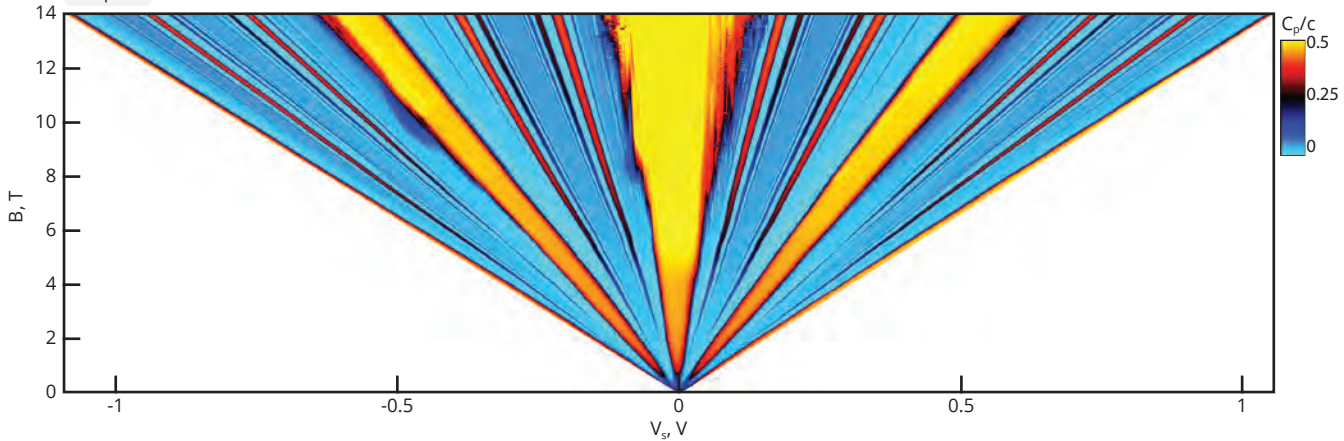

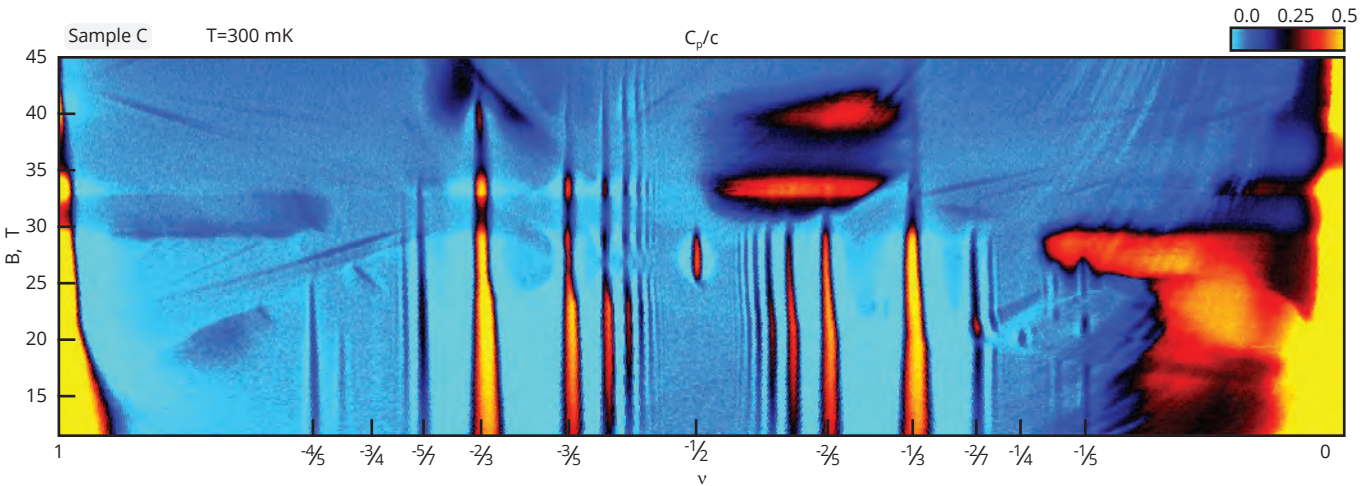

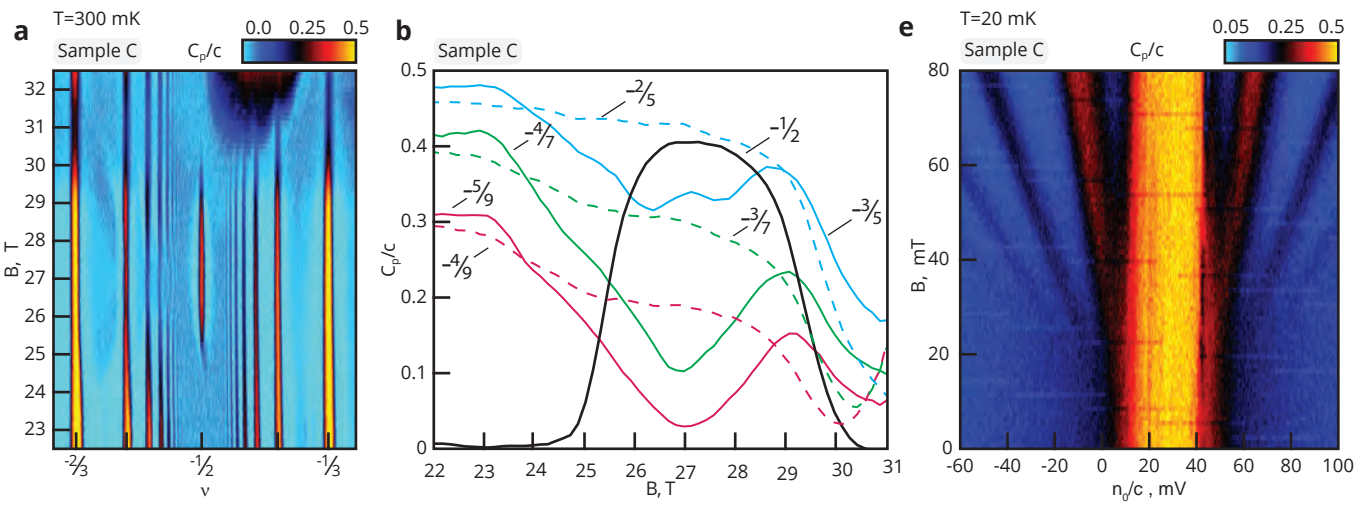

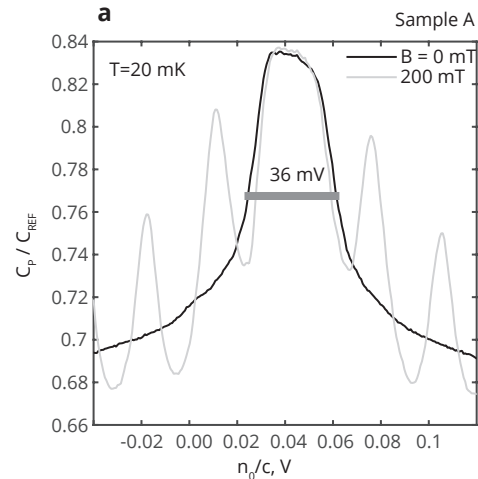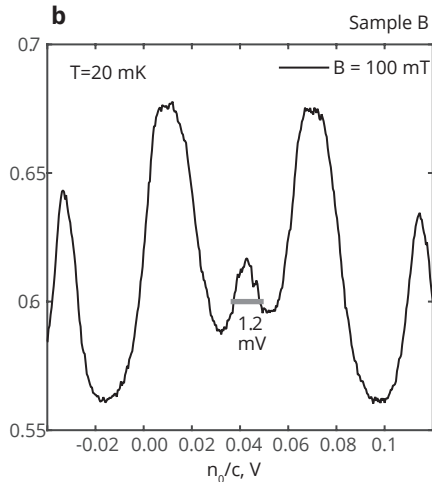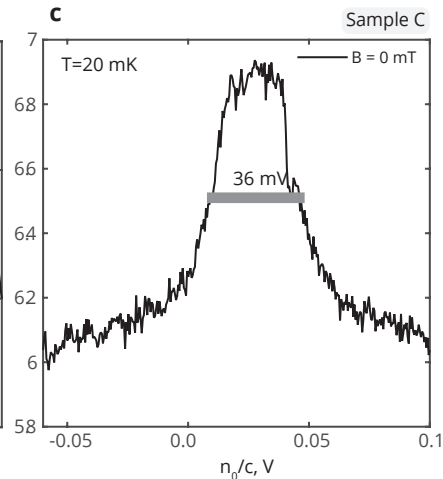



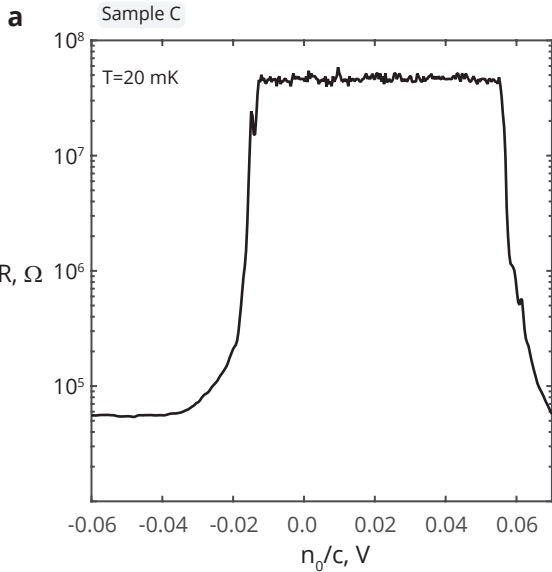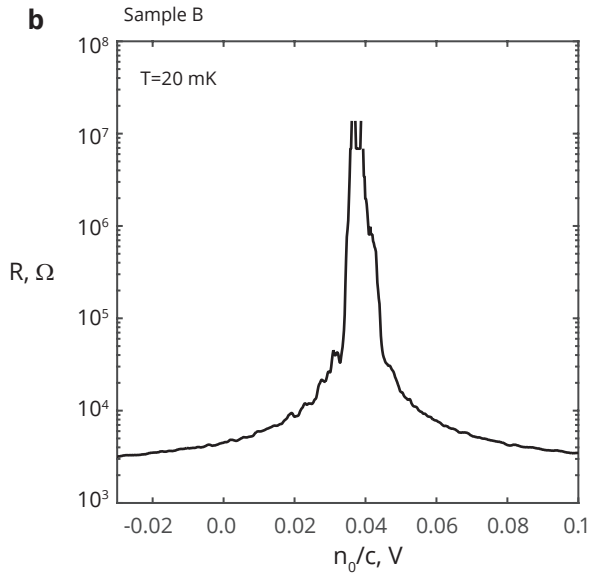

**a**

Sample A

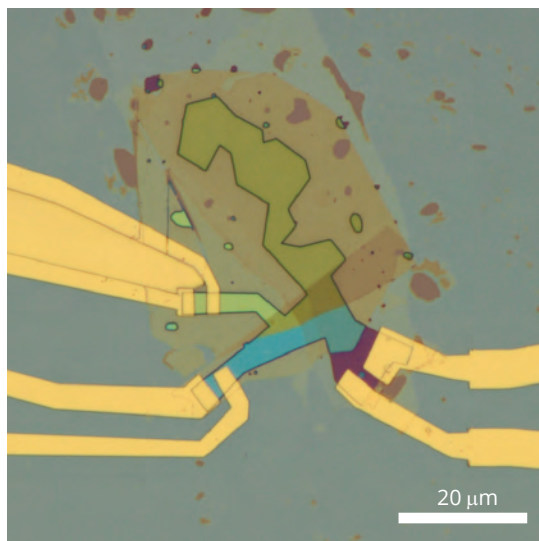**b**

Sample B

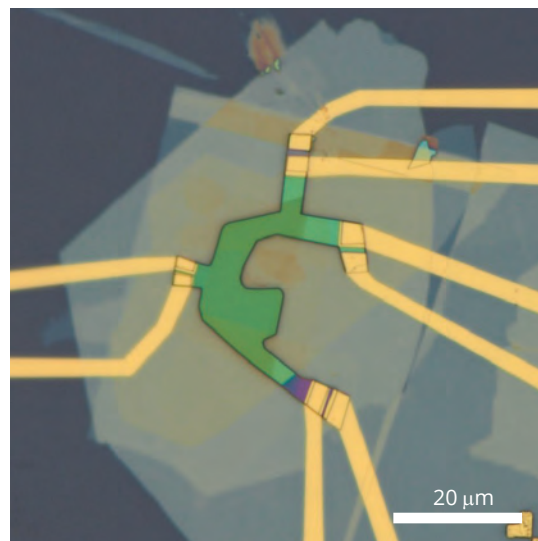**c**

Sample C

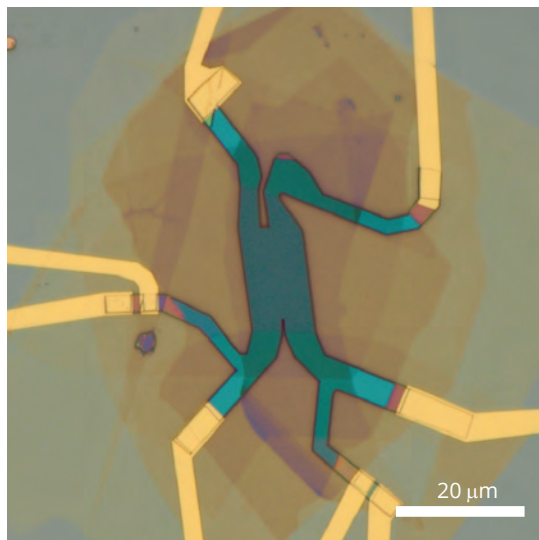**d**

Sample D

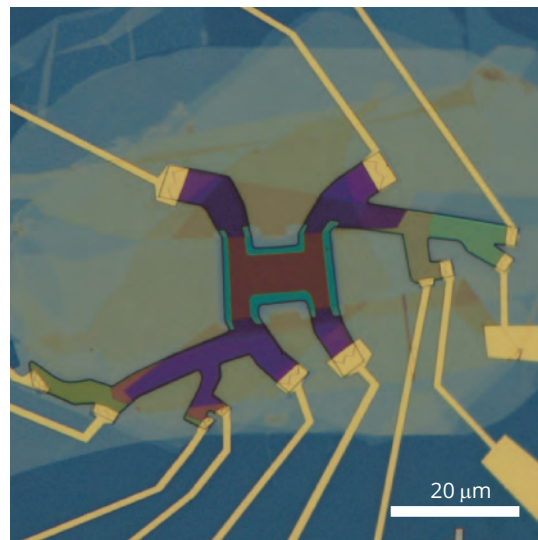

Supplement: Supplementary file 1 [file SuppFigsv4_lowres.pdf]
